# Supplementary material for: Vision Language Model is NOT All You Need: Augmentation Strategies for Molecule Language Models
Source: arXiv:2407.09043 source file (2024-07-23)
Supplement: Supplementary file 1 [file appendix_experiments.tex]

\subsection{Zero-Shot Cross-Modal Retrieval}
\label{app: Zero-Shot Cross-Modal Retrieval}

\noindent \textbf{Complete Set of Experimental Results.}
In this section, we provide a complete set of experimental results for the zero-shot cross-modal retrieval task.
In Table \ref{app tab: cross retrieval full}, we provide empirical results on the (a) description, (b) pharmacodynamics, and (c) ATC dataset.
We observe that as tasks get harder, i.e., increase in the number of options from 4 to 20, the performance disparity between baseline methods and \proposed~broadens.

\begin{table}[t]
\centering
    \resizebox{0.9\linewidth}{!}{
    \begin{tabular}{lccccccc}
    \toprule
    & Aug- & $S^2P$ & $ER$ & & \multirow{2}{*}{Descr.} & \multirow{2}{*}{Pharma.} & \multirow{2}{*}{ATC} \\
    & ment & Loss & Loss & &  &  &  \\
    \midrule
    Ablation 2 & \cmark & \cmark & \xmark & & 96.65 & 80.47 & 51.55 \\
    Ablation 3 & \cmark & \xmark & \cmark & & 96.02 & 78.83 & 51.85 \\
    Ablation 4 & \xmark & \cmark & \cmark & & 96.69 & 79.78 & 50.35 \\
    \midrule
    \proposed & \cmark & \cmark & \cmark & & \textbf{96.84} & \textbf{80.79} & \textbf{53.12} \\
    \bottomrule
    \end{tabular}}
    \caption{Additional ablation studies.}
    \label{app tab: ablation studies}
\end{table}

\begin{table*}[t!]
    \centering
    \resizebox{0.95\linewidth}{!}{
    \begin{tabular}{c|c|ccc|c}
    \toprule
    \multirow{2}{*}{\textbf{Dataset}} & \multirow{2}{*}{\textbf{Prompt}} & \multicolumn{3}{c|}{\textbf{Model}} & \multirow{2}{*}{Random} \\
    \cmidrule{3-5}
    &  & MoMu & MoleculeSTM & \proposed & \\
    \midrule
    \multirow{3}{*}{\textbf{HIA}} & \textcolor{Blue}{Human intestinal absorption (HIA)} & 72.00 & 70.00 & \textbf{92.00} & \multirow{3}{*}{86.50} \\
    \cmidrule{2-5}
    & \multirow{2}{*}{\textcolor{BrickRed}{The molecule is positive w.r.t. a property that is defined as the ability of the body $\cdots$}} & 86.00 & 76.00 & \textbf{92.00} &  \\
    &  & \footnotesize{(+19.44\%)} & \footnotesize{(+8.57\%)} & \footnotesize{(-)} &  \\
    \midrule
    \multirow{3}{*}{\textbf{Pgp Inhibition}} & \textcolor{Blue}{P-glycoprotein Inhibition} & 76.00 & 83.00 & \textbf{97.00} & \multirow{3}{*}{53.36} \\
    \cmidrule{2-5}
    & \multirow{2}{*}{\textcolor{BrickRed}{This molecule is known to inhibit P-glycoprotein, which is an ABC transporter $\cdots$}} & 85.00 & 89.00 & \textbf{96.00} &  \\
    &  & \footnotesize{(+11.84\%)} & \footnotesize{(+7.22\%)} & \footnotesize{(-1.03\%)} &  \\
    \midrule
    \multirow{3}{*}{\textbf{DILI}} & \textcolor{Blue}{Inducing liver injury} & 34.00 & 49.00 & \textbf{56.00} & \multirow{3}{*}{49.68} \\
    \cmidrule{2-5}
    & \multirow{2}{*}{\textcolor{BrickRed}{This molecule induces liver injury that is most commonly caused by Amoxicillin $\cdots$}} & 61.00 & 67.00 & \textbf{76.00} &   \\
    &  & \footnotesize{(+79.41\%)} & \footnotesize{(+36.73\%)} & \footnotesize{(+35.71\%)} &  \\
    \midrule
    \multirow{3}{*}{\textbf{VDR}} & \textcolor{Blue}{Vitamin D receptor} & \textbf{10.00} & \textbf{10.00} & \textbf{10.00} & \multirow{3}{*}{6.14} \\
    \cmidrule{2-5}
    & \multirow{2}{*}{\textcolor{BrickRed}{This molecule is active w.r.t. Vitamin D receptor. The best pharmacophore $\cdots$}} &8.00 & 5.00 & \textbf{11.00} &  \\
    &  & \footnotesize{(-20.00\%)} & \footnotesize{(-50.00\%)} & \footnotesize{(+10.00\%)} &  \\
    \midrule
    \multirow{3}{*}{\textbf{Bioavailability}} & \textcolor{Blue}{Oral Bioavailability} & 82.00 & 93.00 & \textbf{88.00} & \multirow{3}{*}{76.88} \\
    \cmidrule{2-5}
    & \multirow{2}{*}{\textcolor{BrickRed}{The molecule is positive w.r.t. a property that is defined as 'the rate and extent $\cdots$}} & 81.00 & 66.00 & \textbf{82.00} &  \\
    &  & \footnotesize{(-1.22\%)} & \footnotesize{(-29.03\%)} & \footnotesize{(-6.82\%)} &  \\
    \midrule
    \multirow{3}{*}{\textbf{BBB}} & \textcolor{Blue}{Blood-Brain Barrier penetration}
 & 94.00 & 90.00 & \textbf{96.00} & \multirow{3}{*}{76.40} \\
    \cmidrule{2-5}
    & \multirow{2}{*}{\textcolor{BrickRed}{The molecule is able to penetrate the Blood-Brain Barrier, which is the protection layer $\cdots$}} & 85.00 & 86.00 & \textbf{88.00} &  \\
    &  & \footnotesize{(-9.57\%)} & \footnotesize{(-4.44\%)} & \footnotesize{(-8.33\%)} &  \\
    \midrule
    \multirow{3}{*}{\textbf{hERG}} & \textcolor{Blue}{hERG Blocker} & 80.00 & 82.00 & \textbf{87.00} & \multirow{3}{*}{68.86} \\
    \cmidrule{2-5}
    & \multirow{2}{*}{\textcolor{BrickRed}{This molecule blocks the hERG, which is crucial for the coordination of the heart's beating.}} & 68.00 & 71.00 & \textbf{78.00} &   \\
    &  & \footnotesize{(-15\%)} & \footnotesize{(-13.41\%)} & \footnotesize{(-10.33\%)} &  \\
    \midrule
    \multirow{3}{*}{\textbf{HIV}} & \textcolor{Blue}{Active against HIV virus} & 2.00 & 1.00 & \textbf{3.00} & \multirow{3}{*}{3.51}\\
    \cmidrule{2-5}
    & \multirow{2}{*}{\textcolor{BrickRed}{This molecule is active against HIV virus. These drugs typically possess $\cdots$}} & 1.00 & 3.00 & \textbf{4.00} &  \\
    &  & \footnotesize{(-50\%)} & \footnotesize{(+200.00\%)} & \footnotesize{(+33.33\%)} &  \\
    \midrule
    \multirow{3}{*}{\textbf{SARS-Cov-2}} & \textcolor{Blue}{Active against SARS-CoV-2 virus} & 5.00 & 5.00 & \textbf{6.00} & \multirow{3}{*}{5.93}\\
    \cmidrule{2-5}
    & \multirow{2}{*}{\textcolor{BrickRed}{This molecule is active against SARS-CoV-2 virus. These drugs typically possess $\cdots$}} & 4.00 & 5.00 & \textbf{7.00} &  \\
    &  & \footnotesize{(-20\%)} & \footnotesize{(-)} & \footnotesize{(+16.67\%)} &  \\
    \midrule
    \end{tabular}}
    \caption{Additional zero-shot virtual screening task results. The numbers in the bracket indicate the performance increase with \textcolor{BrickRed}{detailed (long)} prompts compared to \textcolor{Blue}{abstract (short)} prompts.}
    \label{app tab: virtual screening}
\end{table*}

\smallskip
\noindent \textbf{Statistical Significance Test.}
To demonstrate the statistical significance of the improvement in Table \ref{tab: cross retrieval}, we performed a paired t-test in the representation learning context for each dataset. 
Since we evaluate models on five independent trials, we compared the mean performances of MoleculeSTM, ablations, and AMOLE across each trial. 
The p-values presented in the table are the outcomes of these paired t-tests, based on the following hypothesis: $H_{0}: \mu_{\text{AMOLE}} = \mu_{\text{Baseline}}$ and $H_{1}: \mu_{\text{AMOLE}} \geq \mu_{\text{Baseline}}$.
In Table \ref{app tab: statistical significance}, we observe that \proposed's improvement over previous works is statistically significance at a p-value of 0.05.

\begin{table}[t]
\centering
    \resizebox{1.00\linewidth}{!}{
    \begin{tabular}{lcccccccc}
    \toprule
    & & \multicolumn{3}{c}{\textbf{Given Molecule @ 20}} & & \multicolumn{3}{c}{\textbf{Given Text @ 20}} \\
    \cmidrule{3-5} \cmidrule{7-9}
    & & Descr. & Pharma. & ATC & & Descr. & Pharma. & ATC \\
    \midrule
    MoMu & & 7.8e-01 & \textbf{5.2e-04} & \textbf{6.5e-06} & & \textbf{1.6e-03} & \textbf{3.9e-05} & \textbf{5.2e-05} \\
    MoleculeSTM (SMILES) & & 5.7e-01 & \textbf{5.9e-04} & \textbf{4.3e-04} & & \textbf{5.1e-04} & \textbf{4.8e-05} & \textbf{3.4e-03} \\
    MoleculeSTM (Graph) & & \textbf{4.3e-03} & \textbf{2.4e-03} & \textbf{3.1e-04} & & \textbf{1.6e-03} & \textbf{2.2e-03} & \textbf{1.4e-05} \\
    \bottomrule
    \end{tabular}}
    \caption{Statistical significance test results. Each number indicates the p-value for the test. Bold indicates the p-values below 0.05.}
    \label{app tab: statistical significance}
\end{table}

Moreover, we also conduct a statistical significance test in ablation studies results in Table \ref{tab: ablation studies} to demonstrate the effectiveness of each component in our model. The p-values detailed in the table are derived from these paired t-tests, underpinning the hypothesis: $H_{0}: \mu_{\text{AMOLE}} = \mu_{\text{Ablation}}$ and $H_{1}: \mu_{\text{AMOLE}} \geq \mu_{\text{Ablation}}$.
From Table \ref{app tab: statistical significance ablation}, we observe that each component of \proposed~statistically significantly contributes to the model performance in the most cases.

\begin{table}[t]
\centering
    \resizebox{1.00\linewidth}{!}{
    \begin{tabular}{lcccccccc}
    \toprule
    & & \multicolumn{3}{c}{\textbf{Given Molecule @ 20}} & & \multicolumn{3}{c}{\textbf{Given Text @ 20}} \\
    \cmidrule{3-5} \cmidrule{7-9}
    & & Descr. & Pharma. & ATC & & Descr. & Pharma. & ATC \\
    \midrule
    MoleculeSTM & & \textbf{4.3e-03} & \textbf{2.4e-03} & \textbf{3.1e-04} & & \textbf{1.6e-03} & \textbf{2.2e-03} & \textbf{1.4e-05} \\
    Ablation1 & & 3.6e-01 & \textbf{4.7e-03} & \textbf{4.7e-03} & & \textbf{9.1e-04} & \textbf{1.3e-02} & \textbf{1.9e-02} \\
    Ablation2 & & 7.3e-01 & \textbf{6.6e-03} & \textbf{3.2e-03} & & \textbf{2.9e-02} & 6.7e-01 & \textbf{3.9e-03} \\
    \bottomrule
    \end{tabular}}
    \caption{Statistical significance test on ablation studies results. Each number indicates the p-value for the test. Bold indicates the p-values below 0.05.}
    \label{app tab: statistical significance ablation}
\end{table}

\smallskip
\noindent \textbf{Model Performance on Dataset Scale.}
In Figure \ref{app fig: dataset scale}, the impact of training data volume on model effectiveness is depicted. 
It's evident that enlarging the training dataset size invariably enhances model efficacy, underscoring the significance of data scale not just in the realm of VLM but equally in MoLM.
We also note that \proposed~uniformly surpasses MoleculeSTM across all data volumes, showcasing \proposed's superior data efficiency.

\smallskip
\noindent \textbf{Additional Ablation Studies.}
In Table \ref{app tab: ablation studies}, we provide further ablation studies to evaluate the effectiveness of each component in \proposed.
As done in Section \ref{sec: Zero-Shot Cross-Modal Retrieval}, we assess the effectiveness of each component by calculating the average performance across hard cross-retrieval tasks, i.e., retrieving among 20 texts given a molecule and retrieving among 20 molecules given a text.
The significance of individual components is observed to change across datasets due to the distinct characteristics of the descriptions they contain. 
Nonetheless, when all elements are integrated, namely in \proposed, it uniformly surpasses a range of simplified models in performance. 
This underlines \proposed's capability to effectively amalgamate different modules for enhanced outcomes.

\smallskip
\noindent \textbf{Sensitivity analysis on $k$.}
In Figure \ref{app fig: sensitivity k}, we illustrate how model performance fluctuates depending on $k$, the hyperparameter that specifies the number of molecules sharing the same description. 
We note that as $k$ is reduced ($k = 10$), the count of molecule-text pairs diminishes, leading to a slight decline in model performance. 
Conversely, as $k$ increases ($k = 100$), the issue of false positives intensifies, suggesting that an optimal level of $k$ needs to be determined during training. 
Despite these variations, we observe that \proposed~consistently surpasses MoleculeSTM across all values of $k$, showcasing the robustness of \proposed~against changes in the hyperparameter $k$.

\begin{figure}[t]
    \centering
    \includegraphics[width=1.0\columnwidth]{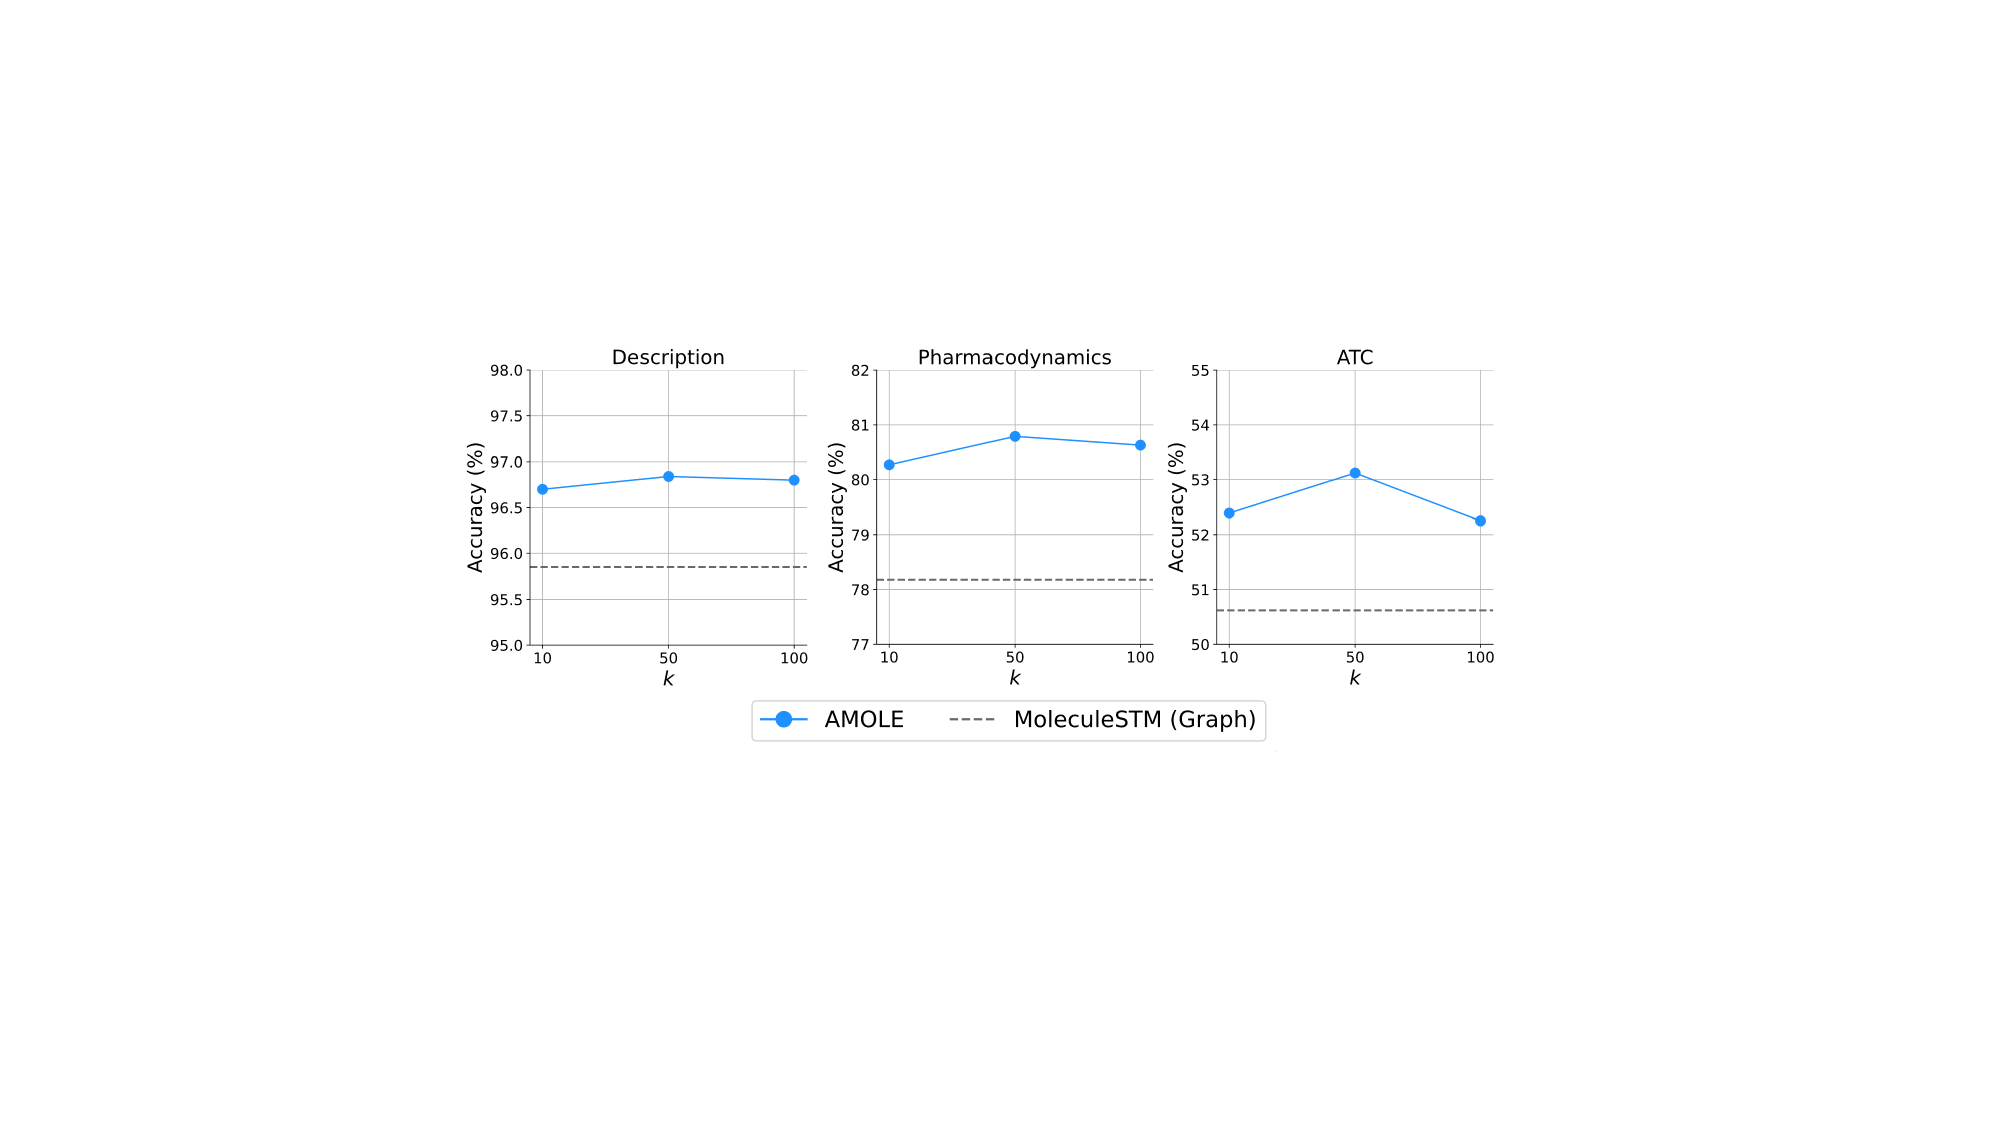} % Reduce the figure size so that it is slightly narrower than the column. Don't use precise values for figure width.This setup will avoid overfull boxes.
    \caption{Sensitivity analysis on $k$.}
    \label{app fig: sensitivity k}
\end{figure}

\subsection{Zero-Shot Question and Answering}
\label{app: Zero-Shot Question and Answering}

In this section, we explore how changes in the input format impact the performance of graph-based baseline models on Zero-Shot question-and-answer tasks. 
Specifically, during training, we randomly replace the input textual description $t_i$ (Original Input) with $\Tilde{t}{i} = $ $t{i}$ \textsf{[SEP]} $t_{i'}$ (Modified Input), which is incorporated for the $ER$ loss in \proposed. 
According to Table \ref{app tab: modified QA}, we see a decline in the performance of baseline models when the input textual description is altered in this manner. 
This suggests that simply concatenating textual descriptions into $\Tilde{t}_{i}$ does not aid the Zero-Shot Question and Answering task, despite their similar input format.
It underscores the need for a more advanced approach, such as expertise reconstruction module in \proposed, to effectively handle QA tasks.

\begin{table}[t]
\centering
    \resizebox{1.00\linewidth}{!}{
    \begin{tabular}{lccccccccc}
    \toprule
    & \multicolumn{2}{c}{\textbf{Original Input}} & & \multicolumn{2}{c}{\textbf{Modified Input}} & \multirow{3}{*}{\proposed} \\
    \cmidrule{2-3} \cmidrule{5-6}
    & \multirow{2}{*}{MoMu} & Molecule & & \multirow{2}{*}{MoMu} & Molecule & \\
    &  & STM & &  & STM  \\
    \midrule
    Descr. & 36.62 & 38.21 & & 36.05 & 37.09 & \textbf{38.61}  \\
    Pharma. & 30.73 & 30.72 &  & 29.57 & 30.58 & \textbf{31.44}  \\
    \bottomrule
    \end{tabular}}
    \caption{Model Performance comparison when the baseline models trained with modified input.}
    \label{app tab: modified QA}
\end{table}

\subsection{Zero-Shot Virtual Screening}
\label{app: Zero-Shot Virtual Screening}

\begin{figure}[t]
    \centering
    \includegraphics[width=0.9\columnwidth]{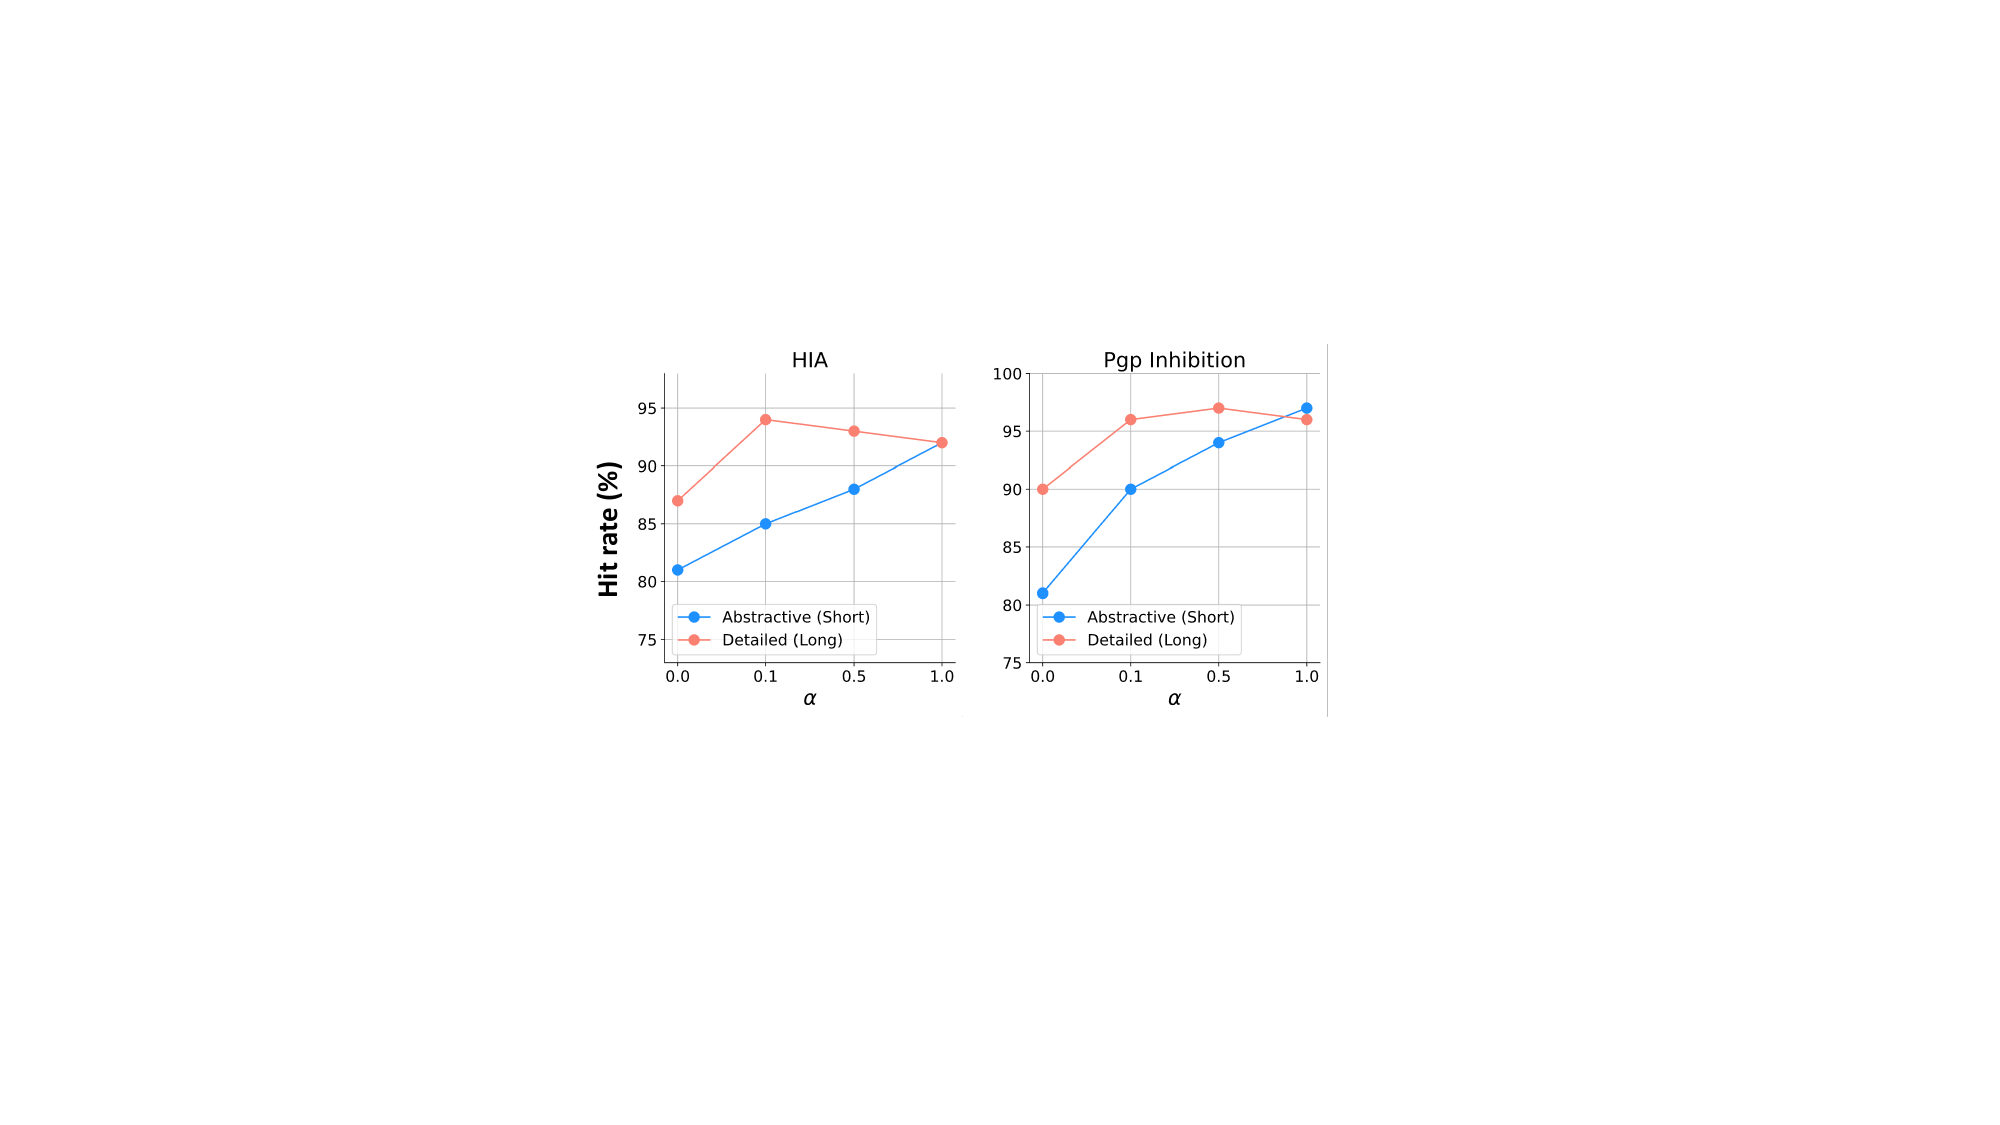} % Reduce the figure size so that it is slightly narrower than the column. Don't use precise values for figure width.This setup will avoid overfull boxes.
    \caption{Sensitivity analysis on $\alpha$.}
    \label{app fig: virtual screening alpha}
    \vspace{-3ex}
\end{figure}

% \begin{figure*}[t!]
%     \centering
%     \includegraphics[width=0.95\textwidth]{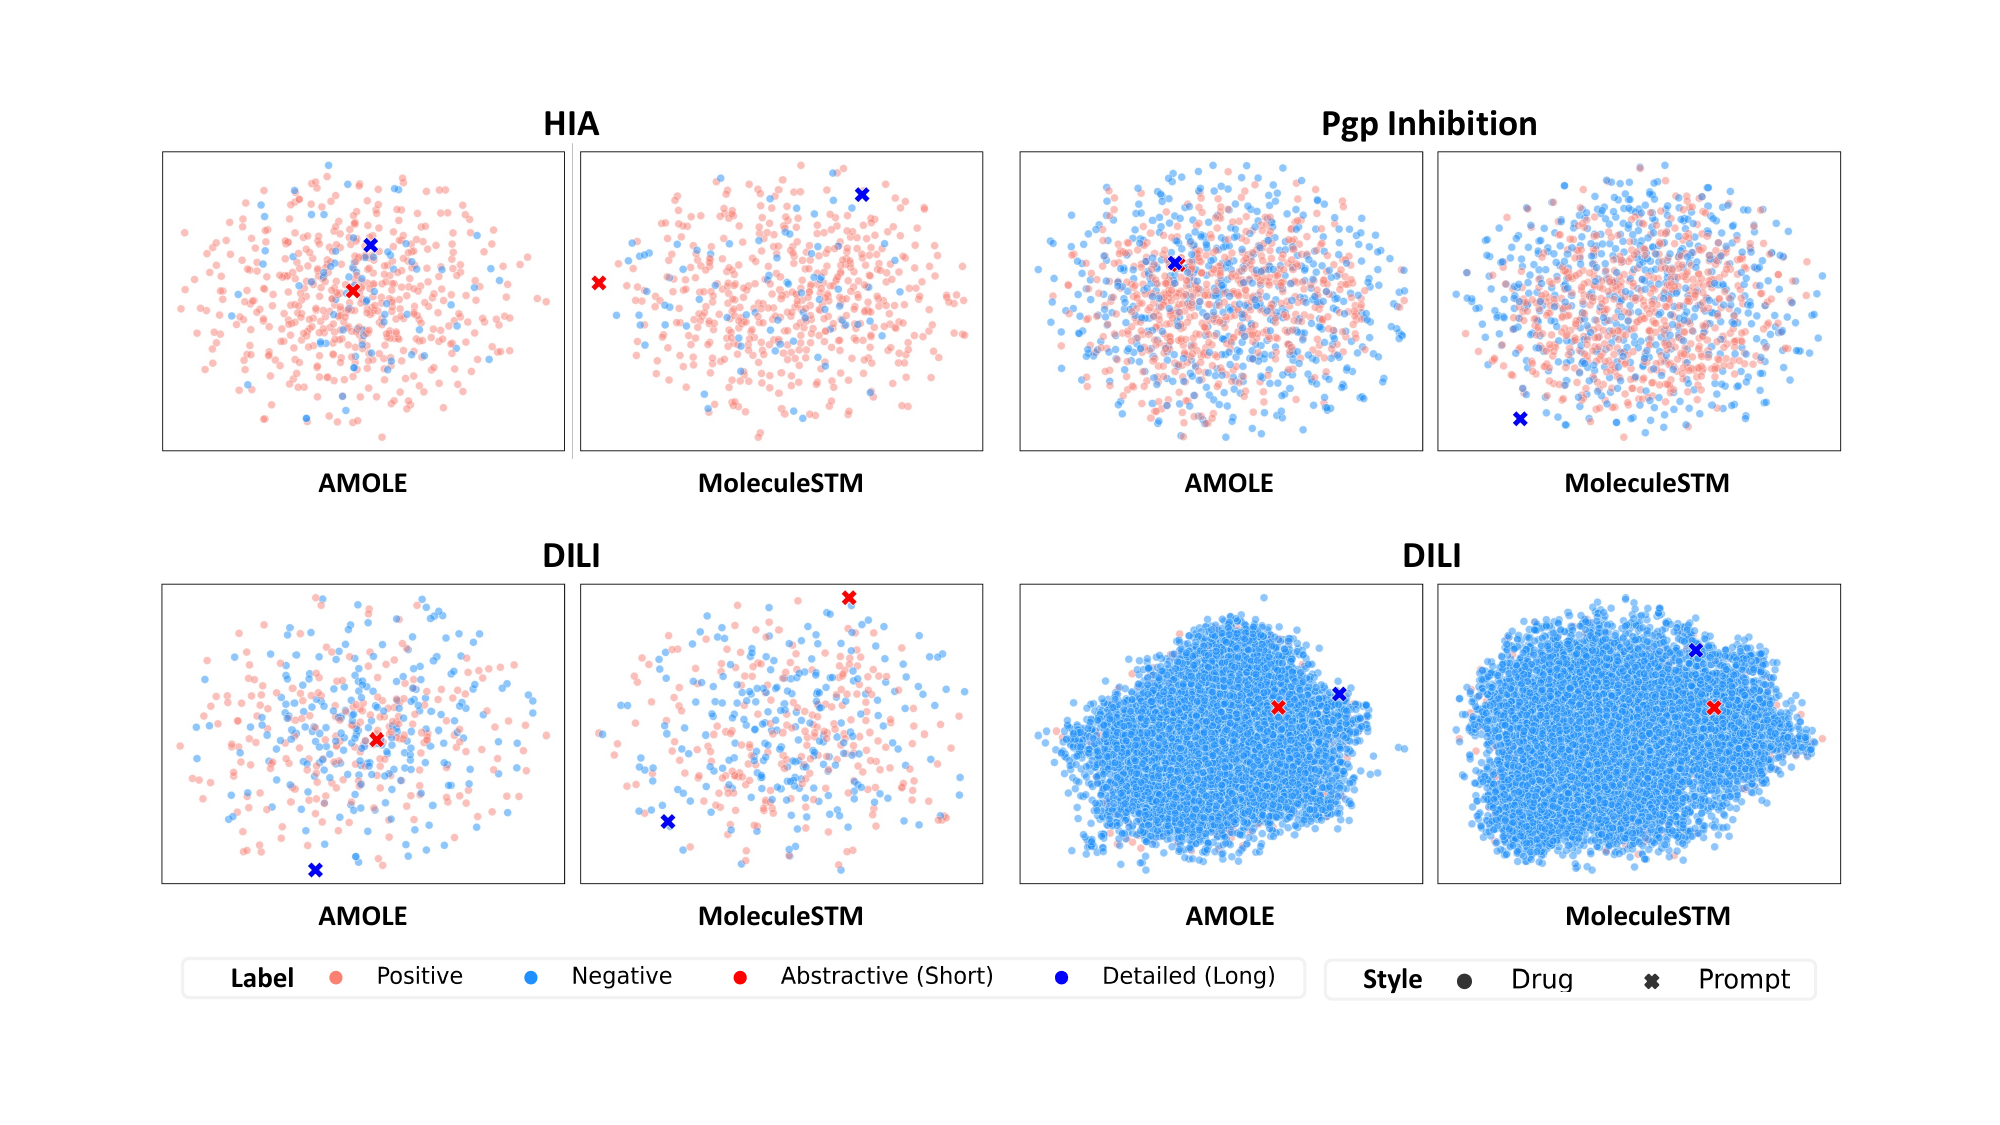} % Reduce the figure size so that it is slightly narrower than the column. Don't use precise values for figure width.This setup will avoid overfull boxes.
%     \caption{Representation space visualization for virtual screening datasets.}
%     \label{app fig: virtual screening representation space}
% \end{figure*}

\noindent \textbf{Additional Experimental Results.}
In this section, we present supplementary experimental outcomes for the zero-shot virtual screening task across multiple datasets. 
As shown in Table \ref{app tab: virtual screening}, it is evident that \proposed~uniformly surpasses the baseline approaches across a range of datasets.
Additionally, it is often noted that the model's efficacy declines when provided with long and detailed descriptions as opposed to short and abstract ones. 
This suggests that detailed prompts are not invariably beneficial, underscoring the significance of the model's resilience across different types of descriptions.

\smallskip
\noindent \textbf{Sensitivity Analysis on $\mathbf{\alpha}$.}
We further investigate the impact of the expertise reconstruction ($ER$) loss weighting factor, $\alpha$, on virtual screening performance. 
It is found that while the model's performance remains largely consistent when provided with a detailed and lengthy prompt, its performance on abstract and brief prompts significantly varies with the choice of $\alpha$. 
Specifically, the model's effectiveness on abstract and concise prompts improves as $\alpha$ increases. 
This suggests that the expertise transfer module effectively allows the model to infer related information, thereby enhancing stability and performance, even when faced with brief and abstract prompts.

% \smallskip
% \noindent \textbf{Qualitative Analysis on Representation Space.}
% In this section, we examine the variation in prompt representation based on its characteristics, i.e., whether it is abstractive (short) or detailed (long). 
% For this purpose, we employ t-SNE \cite{van2008visualizing} visualization to depict the representation of drugs in the dataset alongside the prompts utilized for virtual screening, as shown in Figure \ref{app fig: virtual screening representation space}.
% We note that the representation of prompts generated by MoleculeSTM exhibits significant variation based on their length, indicating that MoleculeSTM's virtual screening effectiveness is greatly influenced by the type of textual description. 
% Conversely, our proposed \proposed~demonstrates a more consistent and stable representation across different prompt types.

\subsection{Effect of $ER$ Loss during training}
\label{app: Effect of ER Loss}

As illustrated by our data analysis in Appendix \ref{app: dataset pre-training}, molecules described by more than two texts are rare, and this scarcity could reduce the effectiveness of the $ER$ Loss.
To analyze the effect of $ER$ loss, we have visualized the change of the $S^2P$ loss and $ER$ loss during training with various levels of $\alpha$.
Figure \ref{app fig: training curve} demonstrates a significant decrease in $ER$ loss as $\alpha$ increases, signifying that the module is capable of efficiently performing expertise reconstruction. 
However, given our main objective is to align molecule and text representations effectively, it is appropriate for the $S^2P$ Loss to play a more substantial role than the $ER$ loss. 
To sum up, we contend that our model adeptly learns the representations of molecules and texts based on structural similarity and enriches the language model through the reconstruction of expertise.

\begin{figure}[t]
    \centering
    \includegraphics[width=0.9\columnwidth]{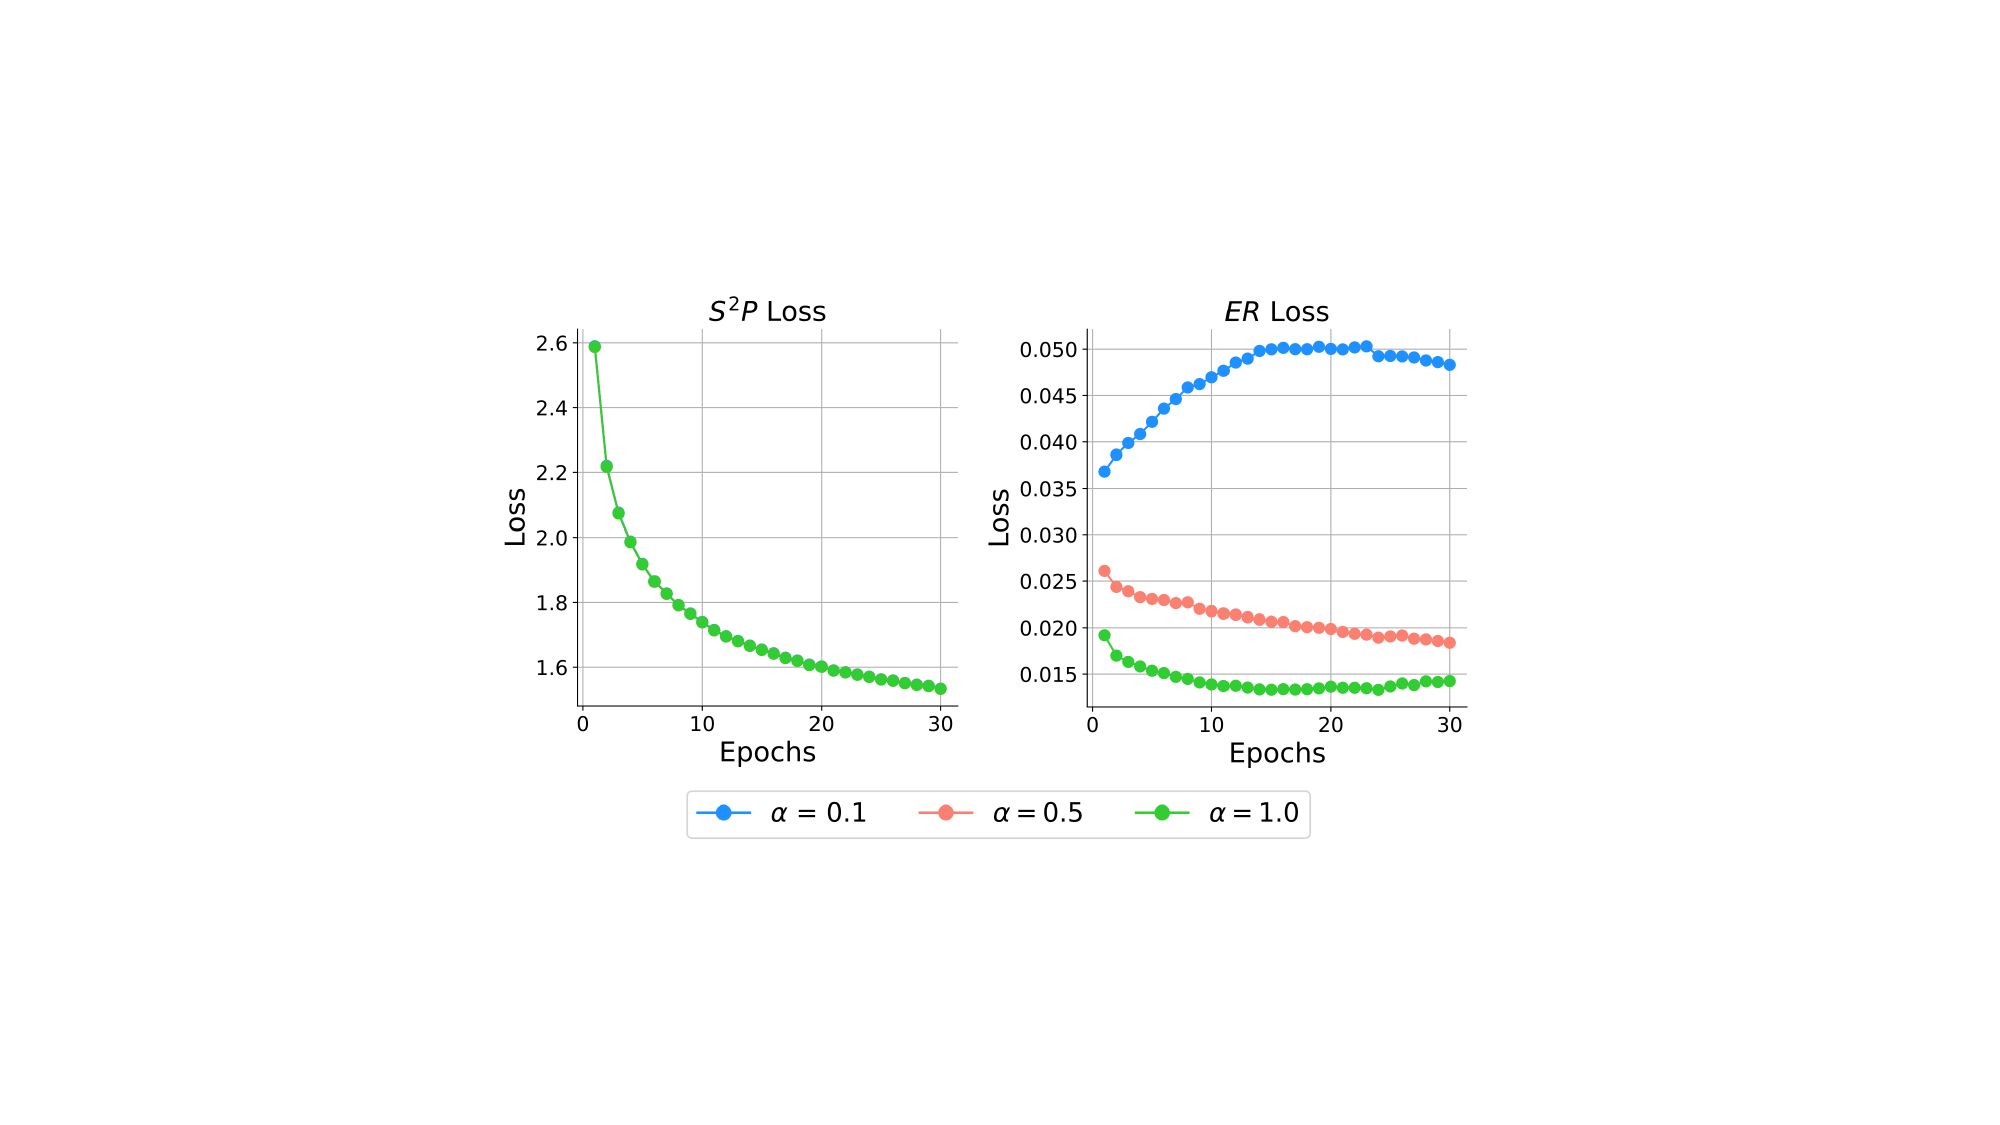} % Reduce the figure size so that it is slightly narrower than the column. Don't use precise values for figure width.This setup will avoid overfull boxes.
    \caption{Training curve in AMOLE.}
    \label{app fig: training curve}
\end{figure}

\section{License for the Datasets}
\label{app: license for the datasets}

\begin{table}[h]
\centering
    \resizebox{0.95\linewidth}{!}{
    \begin{tabular}{c|c}
    \toprule
    \textbf{Dataset} & \textbf{License URL}\\
    \midrule
    PubChem &  \url{https://www.nlm.nih.gov/web_policies.html} \\
    MoleculeNet &  \url{https://opensource.org/license/mit/} \\
    DrugBank &  \url{https://creativecommons.org/licenses/by-nc/4.0/legalcode.en} \\
    TDC &  \url{https://opensource.org/license/mit/} \\
    \bottomrule
    \end{tabular}}
    \caption{Licenses for the datasets used in the paper}
    \label{app tab: license}
\end{table}

In Table \ref{app tab: license}, we detail the sources and data rights for all data components used in this paper.
All data sources underwent thorough examination to confirm that their licensing agreements allow for the type of research we conducted and its further applications.

Throughout the paper, we believe we have properly attributed the creators of the scientific artifacts cited.
We affirm that all data utilized in this study adhere to the conditions of the CC BY 4.0 License. 
We accept the obligation to promote transparent and equitable data usage, acknowledging the original creators' efforts. 
Furthermore, we guarantee that our dataset is free of personally identifiable or privacy-sensitive information.
